# Supplementary material for: LMME3DHF: Benchmarking and Evaluating Multimodal 3D Human Face Generation with LMMs
Source: arXiv:2504.20466 source file (2025-08-05)
Supplement: Supplementary file 1 [file 1_generation_model.tex]

\section{Detailed Information of 3D Human Faces Generation Models }
\label{appendix_1}
\begin{table*}[t]
\centering
  \caption{An overview and URLs of the 3D human faces generation models.}
  \label{model_url}
  % \vspace{-2mm}
    
  \resizebox{0.9\textwidth}{!}{
    \begin{tabular}{l|c|c|c}
    \toprule
     Models & Year & Resolution & URL
     \\
    \midrule 
    EG3D~\cite{chan2022efficient} & 2022 & 512$\times$512 & \url{https://github.com/NVlabs/eg3d}
    \\
    PanoHead~\cite{an2023panohead} & 2023 & 1024$\times$1024 & \url{https://github.com/SizheAn/PanoHead}
    \\
    Next3D~\cite{sun2023next3d} & 2023 & 1024$\times$1024 & \url{https://github.com/MrTornado24/Next3D}
    \\
    AniFaceGAN~\cite{wu2022anifacegan} & 2022 & 512$\times$512 & \url{https://github.com/YueWuHKUST/AniFaceGAN}
    \\
    AniPortraitGAN~\cite{wu2023aniportraitgan} & 2023 & 512$\times$512 & \url{https://github.com/YueWuHKUST/AniPortraitGAN}
    \\
    Portrait4D~\cite{deng2024portrait4d} & 2024 & 1024$\times$1024 & \url{https://github.com/YuDeng/Portrait-4D}
    \\
    Portrait4D-v2~\cite{deng2024portrait4dv2} & 2024 & 1024$\times$1024 & \url{https://github.com/YuDeng/Portrait-4D}
    \\
    StyleSDF~\cite{or2022stylesdf} & 2022 & 1024$\times$1024 & \url{https://github.com/royorel/StyleSDF}
    \\
    VoxGRAF~\cite{schwarz2022voxgraf} & 2022 & 512$\times$512 & \url{https://github.com/autonomousvision/voxgraf}
    \\
    MVCGAN~\cite{zhang2022multi} & 2022 & 1024$\times$1024 & \url{https://github.com/Xuanmeng-Zhang/MVCGAN}
    \\
    cGOF~\cite{sun2022controllable} & 2022 & 512$\times$512 & \url{https://github.com/keqiangsun/cGOF}
    \\
    \bottomrule
  \end{tabular}}
    % \vspace{-3mm}
\end{table*}

\noindent 
{\bf EG3D}~\cite{chan2022efficient}, developed by NVIDIA and Stanford, advances 3D-consistent human face generation by integrating an efficient tri-plane hybrid representation with a StyleGAN2 backbone. It decouples 2D feature generation from neural volume rendering, enabling real-time synthesis of high-resolution, multi-view-consistent images. Through dual discrimination and pose-conditioned generation, EG3D improves geometric fidelity and expression consistency, producing photorealistic 3D human faces from single-view 2D images without requiring multi-view supervision.

\noindent 
{\bf PanoHead}~\cite{an2023panohead} enables 360° geometry-aware synthesis of full human heads from single-view images using only in-the-wild unstructured data. Building on EG3D, PanoHead introduces a tri-grid scene representation to overcome projection ambiguity and mirroring artifacts common in tri-plane-based models. A foreground-aware tri-discriminator decouples the background and enhances geometric fidelity, while a novel two-stage alignment with self-adaptive camera refinement ensures consistent training across wide pose variations. 

\noindent 
{\bf Next3D}~\cite{sun2023next3d} introduces a generative 3D-aware GAN framework capable of animating photorealistic human head avatars with fine-grained control over full-head pose, expressions, gaze, and eye blinks. Leveraging a novel Generative Texture-Rasterized Tri-plane representation, the model combines mesh-guided explicit deformation with implicit volumetric rendering, capturing both facial details and topological variations such as hair or glasses. A style-modulated UNet synthesizes the mouth interior, while a separate tri-plane branch models static components like hair and background. A deformation-aware discriminator ensures expression accuracy and identity preservation. 

\noindent 
{\bf AniFaceGAN}~\cite{wu2022anifacegan} introduces an animatable 3D-aware generative model capable of synthesizing high-quality human face images with disentangled control over pose and expression. Built upon the generative radiance manifolds (GRAM) framework, it decomposes the 3D representation into a template radiance field for identity and an expression-driven deformation field for animation. To enhance realism and consistency, AniFaceGAN employs 3D-space imitation learning with a parametric 3D face model, enforcing geometric alignment through dense shape, landmark, and deformation constraints. 

\noindent 
{\bf AniPortraitGAN}~\cite{wu2023aniportraitgan} introduces the first animatable 3D-aware GAN for portrait synthesis with controllable facial expression, head pose, and shoulder movements. Built upon generative radiance manifolds, the model incorporates 3D morphable face models and the SMPL body model to disentangle identity, expression, and pose. A novel dual-camera rendering scheme and multi-discriminator training framework significantly enhance face fidelity and full-head consistency, while a deformation processing module mitigates artifacts in complex regions like long hair. 

\noindent 
{\bf Portrait4D}~\cite{deng2024portrait4d} presents a one-shot 4D head synthesis framework that reconstructs photorealistic, animatable 3D human heads with full motion control using only synthetic data. The method introduces GenHead, a part-wise 4D generative model trained via adversarial learning on monocular images, which synthesizes large-scale multi-view data with full head, eye, mouth, and neck motion control. Leveraging this data, Portrait4D employs a transformer-based animatable tri-plane reconstructor to produce high-fidelity 4D NeRFs from single images. A novel disentangled learning strategy isolates 3D reconstruction from reenactment to enhance generalizability to real images. 

\noindent 
{\bf Portrait4D-v2}~\cite{deng2024portrait4dv2} proposes a novel learning paradigm for one-shot 4D head avatar synthesis by creating pseudo multi-view videos from monocular inputs. Instead of relying on limited and often inaccurate 3D morphable model (3DMM) reconstructions, the method first trains a static 3D head synthesizer using synthetic multi-view data, which is then employed to generate multi-view sequences from real monocular videos. These pseudo multi-view videos serve as supervision for a transformer-based 4D head generator, trained via cross-view self-reenactment to disentangle expression and pose.

\noindent 
{\bf StyleSDF}~\cite{or2022stylesdf} introduces a high-resolution, 3D-consistent image and geometry generation framework trained solely on single-view images. It combines a signed distance field (SDF)-based implicit volume renderer with a StyleGAN2-based 2D generator, enabling the synthesis of 1024×1024 RGB images along with detailed, view-consistent 3D surfaces. The system renders low-resolution volumetric features, which are then upsampled to high resolution via a styled generator, maintaining identity and geometric consistency across viewpoints. 

\noindent 
{\bf VoxGRAF}~\cite{schwarz2022voxgraf} presents a fast and 3D-consistent generative framework for image synthesis using sparse voxel grids. Unlike prior approaches relying on coordinate-based MLPs, VoxGRAF replaces them with efficient 3D CNNs, enabling single-pass 3D scene generation followed by rapid rendering from arbitrary viewpoints. The method employs a foreground–background disentanglement strategy, combining volumetric rendering with alpha composition, and integrates pruning, progressive growing, and depth-variance regularization to optimize grid sparsity and rendering speed.

\noindent 
{\bf MVCGAN}~\cite{zhang2022multi} introduces a geometry-constrained 3D-aware generative framework that explicitly enforces multi-view consistency in image synthesis. To resolve shape-radiance ambiguity common in NeRF-based models, MVCGAN leverages stereo correspondence and joint optimization across views using image- and feature-level reprojection losses. A hybrid MLP–CNN architecture disentangles 3D shape from 2D appearance, enabling high-resolution image generation with fine detail and consistent geometry. The proposed stereo mixup module enhances realism without additional discriminators, while the two-stage training strategy progressively improves both structural accuracy and visual fidelity.

\noindent 
{\bf cGOF}~\cite{sun2022controllable} introduces a NeRF-based controllable 3D face synthesis framework that enables precise manipulation of shape, expression, and pose from single-view 2D images. At its core is the Conditional Generative Occupancy Field (cGOF), which imposes explicit 3D conditions from 3D Morphable Models (3DMMs) via a mesh-guided volume sampler and a distance-aware density regularizer. To enhance fine-grained control, the framework incorporates a 3D landmark loss and a volume warping loss that enforce semantic and structural consistency across expressions and views.
