# Supplementary material for: LMME3DHF: Benchmarking and Evaluating Multimodal 3D Human Face Generation with LMMs
Source: arXiv:2504.20466 source file (2025-08-05)
Supplement: Supplementary file 2 [file 2_subjective_experiment.tex]

\section{More Details of Subjective Experiment}
\label{appendix_2}

\subsection{Annotaion Dimension}
To comprehensively assess the performance of 3D human face generation models, we propose a dual-dimensional evaluation framework that simultaneously evaluates perceptual quality and authenticity. This approach facilitates a more thorough analysis of both visual fidelity and structural realism, offering a holistic understanding of each model’s strengths and limitations.

\textbf{Perceptual quality:} \quad evaluates the visual fidelity and aesthetic appeal of AI-generated 3D human faces. It emphasizes aspects such as visual clarity (the sharpness and resolution of facial features), naturalness (the realism of skin texture, lighting, and color rendering), and aesthetic appeal (the balance, composition, and expressiveness of facial presentation). High-scoring faces exhibit clean, detailed textures, vivid and harmonious colors, and well-rendered facial elements that contribute to an engaging and visually pleasing appearance. Low-quality outputs often suffer from blurring, faded textures, poor shading, or unnatural color tones that reduce visual impact.

\textbf{Authenticity:} \quad measures how convincingly a generated 3D face mimics a real human, focusing on structural plausibility, identity coherence, and behavioral realism. This includes the anatomical correctness of facial geometry, realistic proportions, believable eye gaze, and subtle expression dynamics such as micro-movements and muscle tension. Unlike perceptual quality, which emphasizes visual polish, authenticity captures whether the face evokes a genuine human presence. High authenticity scores reflect outputs that are not only anatomically sound but also socially and psychologically believable, while low scores indicate artificiality, stiffness, or uncanny features.

\subsection{Significance of the Two Dimensions}
\begin{figure*}[t]
    \centering
    % \vspace{-5mm}
    \includegraphics[width=0.9\textwidth]{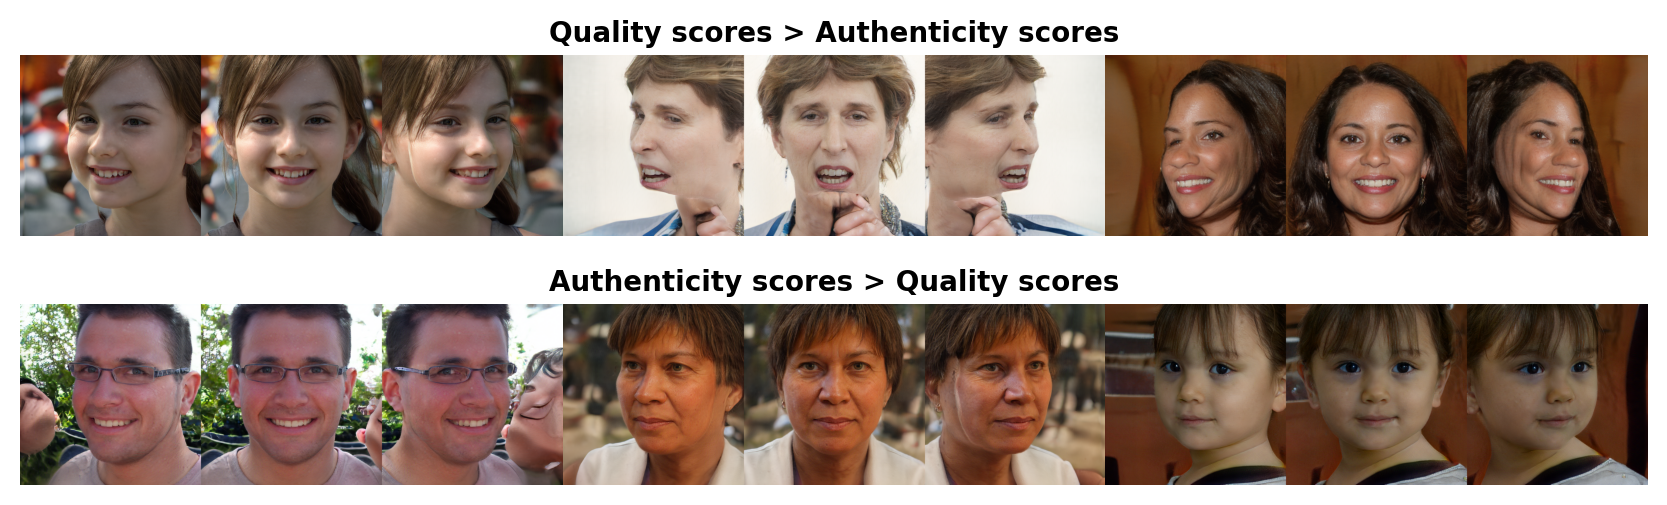}
    % \vspace{-6mm}
    \caption{Illustration of the evaluation dimensions: perceptual quality and authenticity, attached with examples with different subjective qualities.} 
     % \vspace{-1mm}
    \label{appendix_example}
\end{figure*}
The dual-dimensional evaluation framework, combining perceptual quality and authenticity, is essential for capturing the complementary aspects of AI-generated 3D human faces. While perceptual quality focuses on the visual fidelity, clarity, and aesthetic appeal of the synthesized faces, authenticity assesses how convincingly the generated faces resemble real humans in terms of structural plausibility, identity coherence, and behavioral realism. Together, these dimensions provide a comprehensive evaluation of both the visual excellence and human-likeness, offering a balanced assessment of the effectiveness and realism of 3D face generation models.

As illustrated in Figure \ref{appendix_example}, a high perception quality score alone does not guarantee semantic accuracy. For example, an image may exhibit exceptional visual quality, characterized by high resolution, vibrant colors, and meticulous detail, yet fail to accurately represent the specific objects, relationships, or attributes described in the text prompt. Conversely, an image may perfectly align with the textual description in terms of content and context but suffer from poor visual quality, such as low resolution, unnatural textures, or inconsistent lighting, which detracts from its overall appeal and usability.

\subsection{Distortion Marks}
\begin{figure}[!h]
    \centering
    \includegraphics[width=\linewidth]{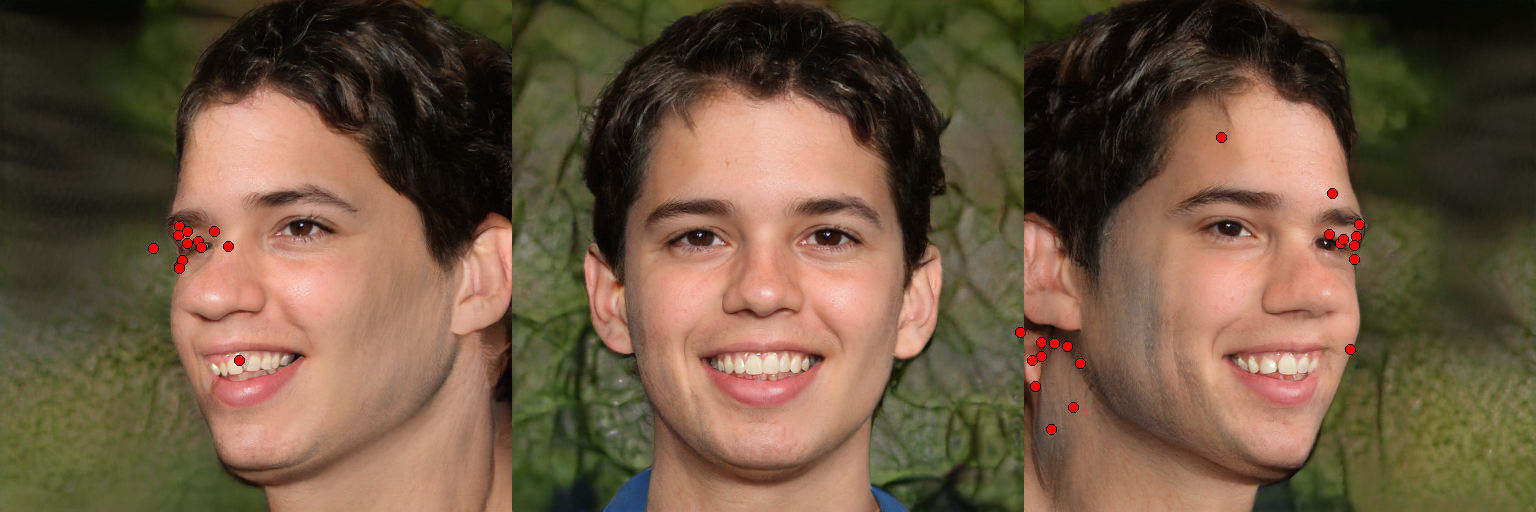}
    \caption{An example of distortion marks.} 
    \vspace{-3mm}
    \label{distortion_sample}
\end{figure}
As part of our subjective experiments, we collected human-marked points on 3D human face renderings to identify perceived distortion regions. As illustrated in Figure \ref{distortion_sample}, the raw annotation data consists of red dots, each representing a click point marked by a participant. To prepare this data for training our saliency decoder, we convert these discrete annotations into continuous grayscale saliency maps using Gaussian filtering. This transformation enables the fixation data to serve as pixel-wise supervision, facilitating the learning of attention-aware representations.

\subsection{Annotation Interface}
\begin{figure*}[t]
	\centering
	\includegraphics[width=0.9\linewidth]{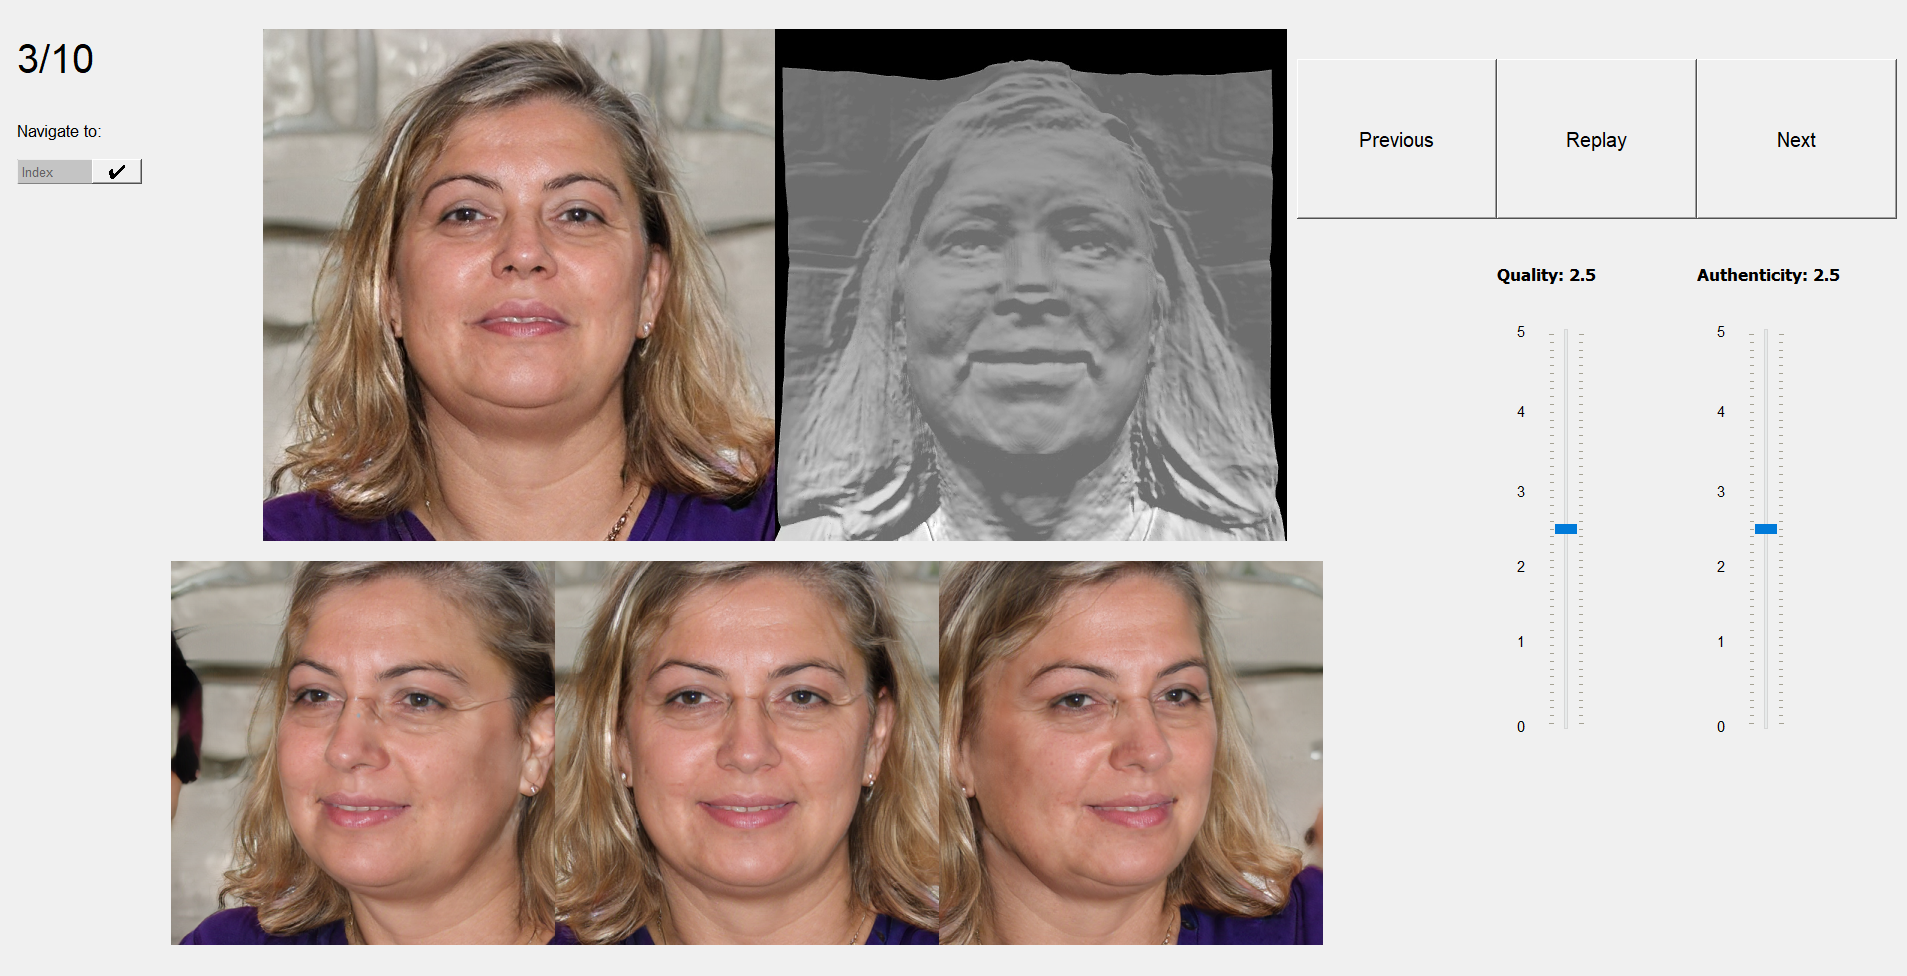}
	\caption{An example of the simple task annotation interface for human evaluation.}
	\label{ui1}
\end{figure*}
\begin{figure*}[!h]
	\centering
	\includegraphics[width=0.9\linewidth]{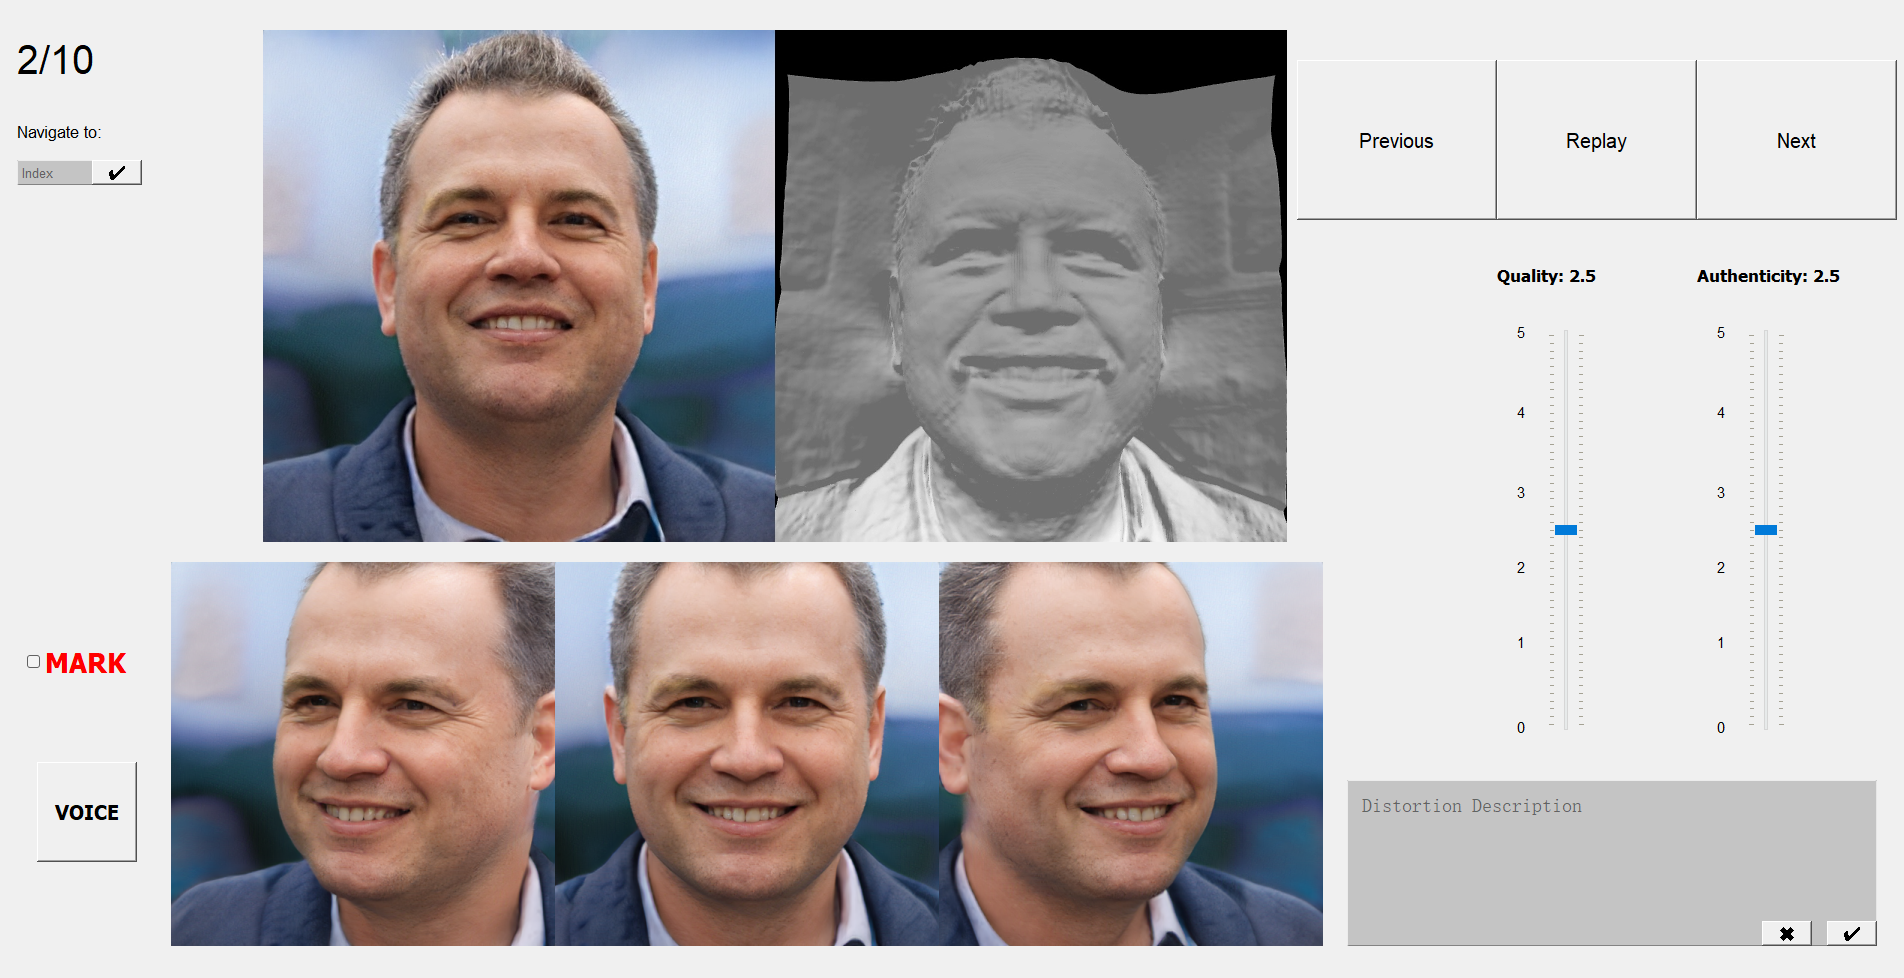}
	\caption{An example of the complex task annotation interface for human evaluation.}
	\label{ui2}
\end{figure*}
To ensure comprehensive and efficient image quality evaluation, we designed two custom annotation interfaces tailored for different assessment tasks: one for simple tasks and another for complex tasks. The simple task annotation interface, shown in Figure \ref{ui1}, is a manual evaluation platform developed using the Python Tkinter package. It is designed to facilitate the collection of Mean Opinion Scores (MOS) by enabling participants to evaluate 3D human faces along two independent dimensions: quality and authenticity. The 3D HF samples presented are randomly selected from ten different generation models.

In contrast, the complex task annotation interface, illustrated in Figure \ref{ui2}, is also developed using the Tkinter package but includes extended functionality for more detailed annotation. This interface is used to determine and mark distortion regions and provide corresponding descriptions. Compared to the simple interface, it incorporates additional tools such as a “MARK” button to activate region marking and a “VOICE” button for recording spoken descriptions. Participants may also enter descriptions manually using the provided text box. The recorded audio is converted into text and, along with manual input, is ultimately displayed in the bottom-right panel of the interface.
