# Supplementary material for: LMME3DHF: Benchmarking and Evaluating Multimodal 3D Human Face Generation with LMMs
Source: arXiv:2504.20466 source file (2025-08-05)
Supplement: Supplementary file 3 [file 3_database.tex]

\section{More Analysis of Gen3DHF Database}
\label{appendix_3}

\subsection{MOS Distribution across 10 Generation Models}
\begin{figure*}[t]
    \centering
    \vspace{-5mm}
    \includegraphics[width=1\textwidth]{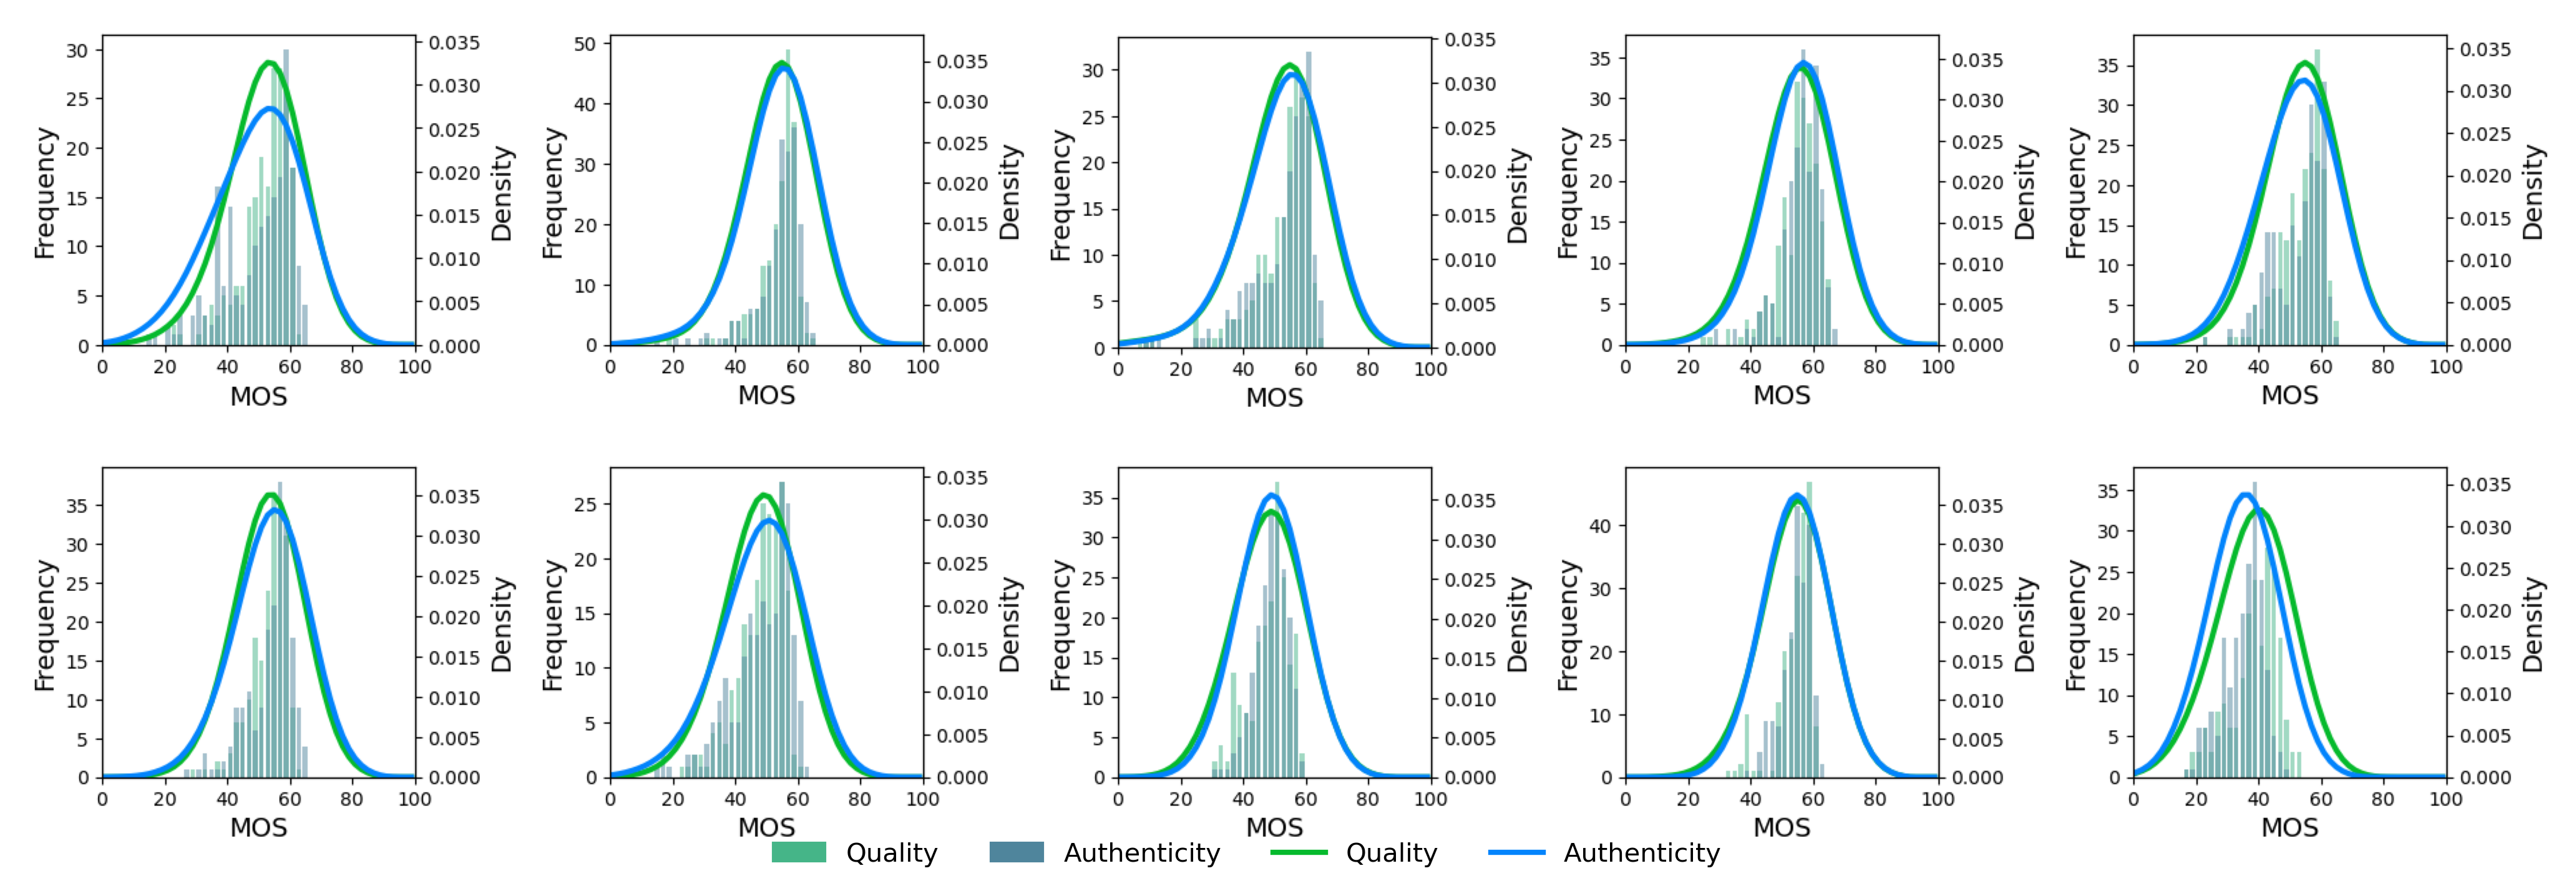}
    \vspace{-6mm}
    \caption{Mean Opinion Score (MOS) distribution histograms and kernel density curves of Gen3DHF dataset. It includes two dimensions: Quality MOS and Authenticity MOS. Each dimension contains a total of 2,000 MOS values.} 
     \vspace{-1mm}
    \label{appendix_mos}
\end{figure*}
As mentioned in the main text, we process and compute the valid subjective evaluation results, obtaining a total of 2,000 Mean Opinion Scores (MOSs) across two dimensions, along with QA accuracy. Figure \ref{appendix_mos} better illustrate the generative capabilities of current 3D HFs generation models, as we plot histograms and kernel density curves (KDC) graphs. The MOS distributions across the 10 generation models reveal generally normal-shaped curves centered between MOS 40 and 70, indicating consistent perceptual ratings. Quality and authenticity scores often overlap, suggesting a strong correlation between visual quality and perceived realism, though some models show slight divergence—implying trade-offs between the two. Variability differs among models, with some exhibiting tighter distributions and others showing broader spreads. Overall, while all models operate within a similar perceptual range, subtle differences in distribution shape and alignment highlight model-specific tendencies toward either realism or refinement.
