# Supplementary material for: LMME3DHF: Benchmarking and Evaluating Multimodal 3D Human Face Generation with LMMs
Source: arXiv:2504.20466 source file (2025-08-05)
Supplement: Supplementary file 4 [file 4_train_loss.tex]

\section{Details of Loss Function}
\label{appendix_4}
The training process for LMME3DHF is divided into three progressive stages, each utilizing a specific loss function to target distinct objectives: language loss for instruction tuning, aligning visual and language features to give visual question answers, L1 loss for quality regression fine-tuning to generate accurate perception and correspondence scores and a linear combine loss for distortion-aware saliency prediction. 

\subsection{Instruction tuning with language loss.}
In the first stage, we train the LLM to align visual and language features using the standard language loss. The language loss, calculated using a cross-entropy function, measures the model’s ability to predict the correct token given the prior context:
\begin{eqnarray}
\begin{aligned}
&\mathcal{L}_{\text{language}} = -\frac{1}{N} \sum_{i=1}^N \log P(y_{\text{label}} | y_{\text{pred}})
\end{aligned}
\end{eqnarray}
where $P(y_{\text{label}} | y_{\text{pred})}$ represents the probability assigned to the correct token $y_{\text{label}}$ by the model, $y_{\text{pred}}$ is the predicted token, and $N$ is the total number of tokens. By minimizing this loss, the model learns to generate coherent textual descriptions of image content, laying the foundation for subsequent stages.

\subsection{Refining quality scoring with L1 loss.}
Once the model can categories the quality class of video content, the focus shifts to fine-tuning the quality regression module to output stable and precise numerical quality scores. The training objective minimizes the difference between the predicted quality score $Q_{predict}$ and the ground-truth MOS  $Q_{label}$ using the L1 loss function:
\begin{eqnarray}
\begin{aligned}
\label{loss_function}
\mathcal{L}_{\text{MOS}} = \frac{1}{N} \sum_{i=1}^N \left| Q_{\text{predict}}(i) - Q_{\text{label}}(i) \right|
\end{aligned}
% \vspace{-3mm}
\end{eqnarray}
where $Q_{\text{predict}}(i)$ is the score predicted by the regressor $i$ and $Q_{\text{label}}(i)$ is the corresponding ground-truth MOS derived from subjective experiments, and $N$  is the number of images in the batch. This loss function ensures that the predicted scores remain consistent with human evaluations, enabling the model to accurately assess the quality of AI-generated 3D human faces in numerical form.

\subsection{Distortion-aware saliency decoder}
In order to generate accurate distortion-aware saliency maps, we design a loss function aimed at maximizing prediction performance. The training loss function for the saliency decoder is defined in Equation (5), which is a linear combination of four loss functions: L1 Loss, Correlation Coefficient Loss, KL Divergence Loss, and Binary Cross-Entropy Loss. 
\begin{equation}
    \mathcal{L} = \omega_{1}\mathcal{L}_{L1} + \omega_{2}\mathcal{L}_{CC} + \omega_{3}\mathcal{L}_{KL} + \omega_{4}\mathcal{L}_{BCE}   
\end{equation}
