# Supplementary material for: LMME3DHF: Benchmarking and Evaluating Multimodal 3D Human Face Generation with LMMs
Source: arXiv:2504.20466 source file (2025-08-05)
Supplement: Supplementary file 5 [file 5_implementions.tex]

\section{Implemention Details}
\label{appendix_5}
\subsection{Detailed Information of Evaluation Criteria}
We adopt the widely used metrics in quality assessment metrics: Spearman rank-order correlation coefficient (SRCC), Pearson linear correlation coefficient (PLCC), and Kendall’s Rank Correlation Coefficient (KRCC) as our evaluation criteria. SRCC quantifies the extent to which the ranks of two variables are related, which ranges [-1, 1]. Given $N$ action images, SRCC is computed as:
\begin{equation}
SRCC = 1 - \frac{{6\sum\nolimits_{n = 1}^N {{{({v_n} - {p_n})}^2}} }}{{N({N^2} - 1)}},
\end{equation}
where $v_n$ and $p_n$ denote the rank of the ground truth $y_n$ and the rank of predicted score ${\hat y_n}$ respectively. The higher the SRCC, the higher the monotonic correlation between ground truth and predicted score.

PLCC measures the linear correlation between predicted scores and ground truth scores, which can be formulated as:
\begin{equation}
PLCC = \frac{{\sum\nolimits_{n = 1}^N {({y_n} - \bar y)({{\hat y}_n} - \bar {\hat y})} }}{{\sqrt {\sum\nolimits_{n = 1}^N {{{({y_n} - \bar y)}^2}} } \sqrt {\sum\nolimits_{n = 1}^N {{{({{\hat y}_n} - \bar {\hat y})}^2}} } }},
\end{equation}
where $\bar y$ and $\bar {\hat y}$ are the mean of ground truth and predicted score respectively.

KRCC measures the ordinal association between two variables. For a pair of ranks $(v_i, p_i)$ and $(v_j, p_j)$, the pair is concordant if:
\begin{equation}
(v_i - v_j)(p_i - p_j) > 0,
\end{equation}
and discordant if $<  $ 0.
% \begin{equation}
% (v_i - v_j)(p_i - p_j) \textless  0.
% \end{equation}
 Given $N$ AIGVs, KRCC is computed as:
\begin{equation}
KRCC =  \frac{{C - D}}{{\frac{1}{2}N(N-1)}},
\end{equation}
where $C$ and $D$ denote the number of concordant and discordant pairs, respectively. 

\subsection{Detailed Information of Evaluation Methods}
\noindent
{\bf CNNIQA}~\cite{kang2014convolutional} is a convolutional neural network (CNN) designed for no-reference image quality assessment (NR-IQA), which predicts the visual quality of distorted images without using reference images. Unlike traditional methods that rely on handcrafted features, CNNIQA directly learns discriminative features from raw image patches, allowing for a more efficient and effective image quality estimation.

\noindent
{\bf StairIQA}~\cite{sun2023blind} employs a staircase structure that hierarchically integrates features from intermediate layers of a CNN, allowing it to leverage both low-level and high-level visual information for more effective quality assessment. Additionally, it introduces an Iterative Mixed Database Training (IMDT) strategy, which trains the model across multiple diverse databases to improve generalization and handle variations in image content and distortions. 

\noindent
{\bf HyperIQA}~\cite{su2020blindly} aims at handling authentically distorted images. It addresses two main challenges: distortion diversity and content variation. The model is based on a self-adaptive hyper network that adjusts quality prediction parameters according to the image content, making the predictions more consistent with human perception. 

\noindent
{\bf Simple-VQA}~\cite{wu2023exploring} proposes an efficient deep learning-based no-reference VQA model tailored for UGC videos by directly learning quality-aware spatial and motion features from raw frames. It introduces a lightweight two-branch architecture—an end-to-end CNN for spatial distortion modeling and a pretrained action recognition network for capturing motion-related quality. The model employs sparse keyframe sampling and low-resolution motion processing to minimize computational overhead, and further enhances performance via a multi-scale quality fusion strategy inspired by the human visual system.

\noindent
{\bf FAST-VQA}~\cite{sun2023blind} proposes a fragment-based sampling strategy that retains both local texture and global scene quality by extracting spatially uniform, temporally aligned mini-patches from videos. It introduces a Fragment Attention Network (FANet) to effectively process these fragments, using gated position biases and non-linear regression for robust quality prediction.

\noindent
{\bf DOVER}~\cite{wu2023exploring} introduces a disentangled video quality assessment framework that separates aesthetic and technical perspectives in user-generated content (UGC) videos. It uses a View Decomposition strategy with two dedicated branches: one capturing high-level semantic aesthetics and the other modeling low-level technical distortions. 

\noindent
{\bf TCSVT-BVQA}~\cite{wu2023exploring} proposes a blind video quality assessment method that combines quality-aware spatial feature pre-training with motion perception from a 3D action recognition model. It transfers knowledge from image quality assessment datasets and Kinetics-400 to learn spatial and temporal features, enabling better generalization to authentic distortions in real-world videos.

\noindent
{\bf VSFA}~\cite{wu2023exploring} introduces a no-reference video quality assessment method designed for in-the-wild videos by modeling two key aspects of the human visual system: content dependency and temporal-memory effects. It extracts content-aware features from a pretrained CNN and models long-term temporal dependencies using a gated recurrent unit (GRU). A subjectively-inspired temporal pooling layer captures the hysteresis effect in human perception, improving alignment with real user preferences.

\noindent
{\bf VideoChat2}~\cite{li2023videochat} introduces a chat-centric video understanding system that integrates video foundation models with large language models through a learnable neural interface. It offers two versions: VideoChat-Text, which textualizes video content using perception models and LLMs, and VideoChat-Embed, which encodes video features directly for multimodal dialogue. A novel video-centric instruction dataset is proposed to enhance spatiotemporal reasoning and causal understanding.

\noindent
{\bf LLaVA-NeXT}~\cite{liu2024llavanext} improves on LLaVA-1.5~\cite{liu2024improved} by increasing input image resolution and enhances visual detail, reasoning, and OCR capabilities. It also improves world knowledge and logical reasoning while maintaining LLaVA's minimalist design and data efficiency, using under 1M visual instruction tuning samples. 

\noindent
{\bf InternVL2.5}~\cite{chen2024expanding} demonstrates strong performance in various benchmarks, including multi-discipline reasoning, document and video understanding, and multimodal hallucination detection. The model features enhanced vision encoders, larger dataset sizes, and improved test-time scaling.

\noindent
{\bf MiniCPM-V2.6}~\cite{yao2024minicpm} is designed for deployment on end-side devices, addressing the challenges of running large models with significant computational costs. Key features include strong OCR capability, supporting high-resolution image perception, trustworthy behavior with low hallucination rates, and multilingual support for over 30 languages. 

\noindent
{\bf Qwen2-VL}~\cite{wang2024qwen2}
is an advanced large vision-language model designed to process images, videos, and text with dynamic resolution handling and multimodal rotary position embedding (M-RoPE). The model features strong capabilities in OCR, video comprehension, multilingual support, and robust agent functionalities for device operations. 

\noindent
{\bf Video-ChatGPT}~\cite{li2023videochat} introduces a multimodal framework for open-ended video conversation by aligning a video-adapted visual encoder with a large language model (LLM). It leverages a novel dataset of 100,000 video-instruction pairs, created through a hybrid human-assisted and semi-automatic annotation pipeline, to enhance temporal understanding and conversational reasoning. By fine-tuning only a lightweight adapter layer, the model captures both spatial and temporal cues, achieving state-of-the-art performance across multiple video QA benchmarks.

\noindent
{\bf Video-LLaVa}~\cite{lin2023video} introduces a unified vision-language framework that aligns image and video representations before projection, enabling large language models to reason over both modalities simultaneously. It leverages LanguageBind encoders to map visual inputs into a shared language feature space and conducts joint training on image and video data for multimodal instruction following.

\noindent
{\bf Video-LLaMA2}~\cite{cheng2024videollama} enhances video-language understanding by introducing a Spatial-Temporal Convolution (STC) connector and an Audio Branch for joint multimodal learning. It processes spatial and temporal dynamics more effectively than previous models and integrates audio cues for enriched video comprehension.

\subsection{Question design for LLM-based models}
For LLM-based detection methods, it is necessary to provide not only the video to be evaluated but also a corresponding prompt to guide the model toward producing the desired output. Specifically, three different questions must be input for each video to enable comprehensive evaluation. The specific question template is as follows:
\begin{itemize}
    \item \textbf{Quality}:
    Please rate the quality of the human face in this video, considering factors such as resolution, clarity, smoothness, and overall visual quality.
    \item \textbf{Authenticity}:
    Please rate the authenticity of the human face in this video, considering factors such as natural facial movements, consistency, texture realism, and any signs of digital manipulation or artificial generation.
    \item \textbf{Dsitortion Description}:
    Examine each angle within the image and identify any noticeable distortions. Choose one or more categories from the following list to classify any distortions you find: Eye Distortions, Mouth Distortions, Hair Distortions, Facial Feature Distortions, Head Structure Distortions, Overlap or Blending Issues, Blurring / Exposure / Grain, Accessories or Cloth Distortions.
\end{itemize}
