# Supplementary material for: LMME3DHF: Benchmarking and Evaluating Multimodal 3D Human Face Generation with LMMs
Source: arXiv:2504.20466 source file (2025-08-05)
Supplement: Supplementary file 6 [file 0_overview.tex]

\section{Overview}
In this supplementary material, we provide additional details regarding the data collection, methodology, experiments, and results presented in the main paper. In Section \ref{appendix_1}, we offer an overview of the 11 3D human face generation models used in our study. Section \ref{appendix_2} elaborates on the subjective experiment setup, including annotation dimensions, evaluation criteria, interface design, and participant management. In Section \ref{appendix_3}, we present an in-depth analysis of the Gen3DHF database, including the distribution of Mean Opinion Scores (MOS) across the 10 generation models. The loss functions used during the training of the LMM4Gen3DHF model are described in Section \ref{appendix_4}. Lastly, Section \ref{appendix_5} provides details on the evaluation criteria and the algorithms employed in our analysis.
