# Supplementary material for: LMME3DHF: Benchmarking and Evaluating Multimodal 3D Human Face Generation with LMMs
Source: arXiv:2504.20466 source file (2025-08-05)
Supplement: Supplementary file 7 [file appendix_example.tex]

\begin{figure*}[t]
    \centering
    % \vspace{-5mm}
    \includegraphics[width=0.9\textwidth]{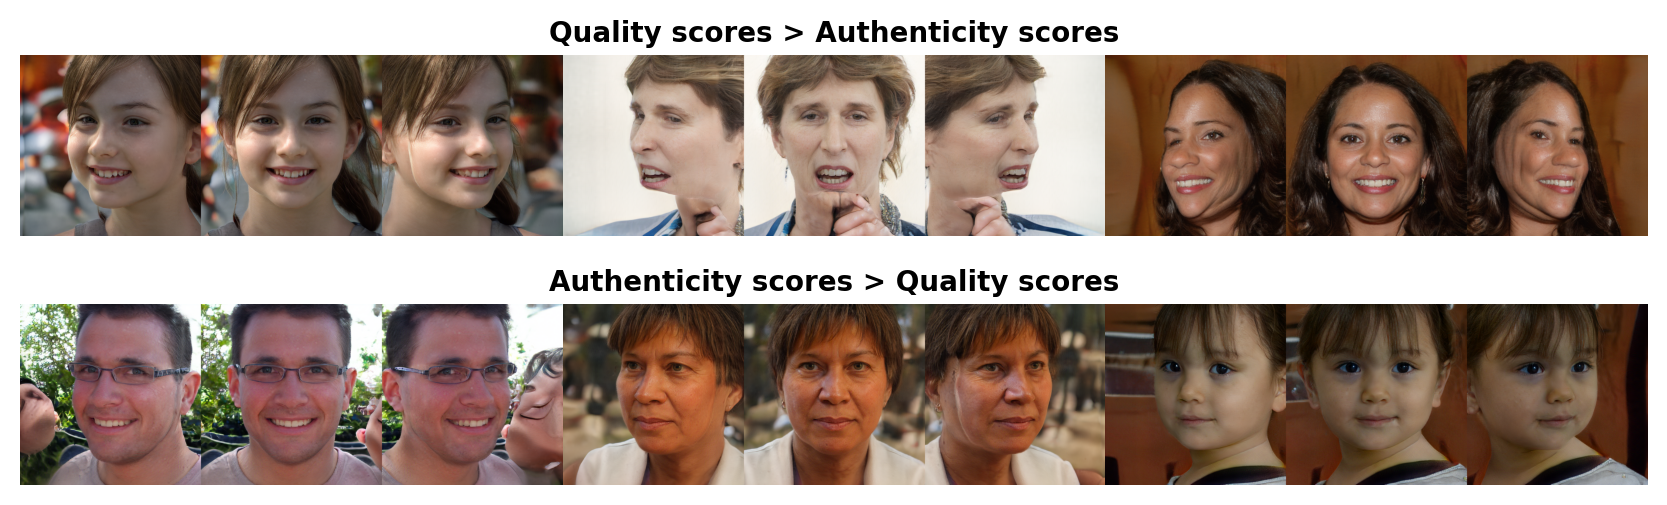}
    % \vspace{-6mm}
    \caption{Illustration of the evaluation dimensions: perceptual quality and authenticity, attached with examples with different subjective qualities.} 
     % \vspace{-1mm}
    \label{appendix_example}
\end{figure*}
