# Supplementary material for: LMME3DHF: Benchmarking and Evaluating Multimodal 3D Human Face Generation with LMMs
Source: arXiv:2504.20466 source file (2025-08-05)
Supplement: Supplementary file 8 [file appendix_mos.tex]

\begin{figure*}[t]
    \centering
    \vspace{-5mm}
    \includegraphics[width=1\textwidth]{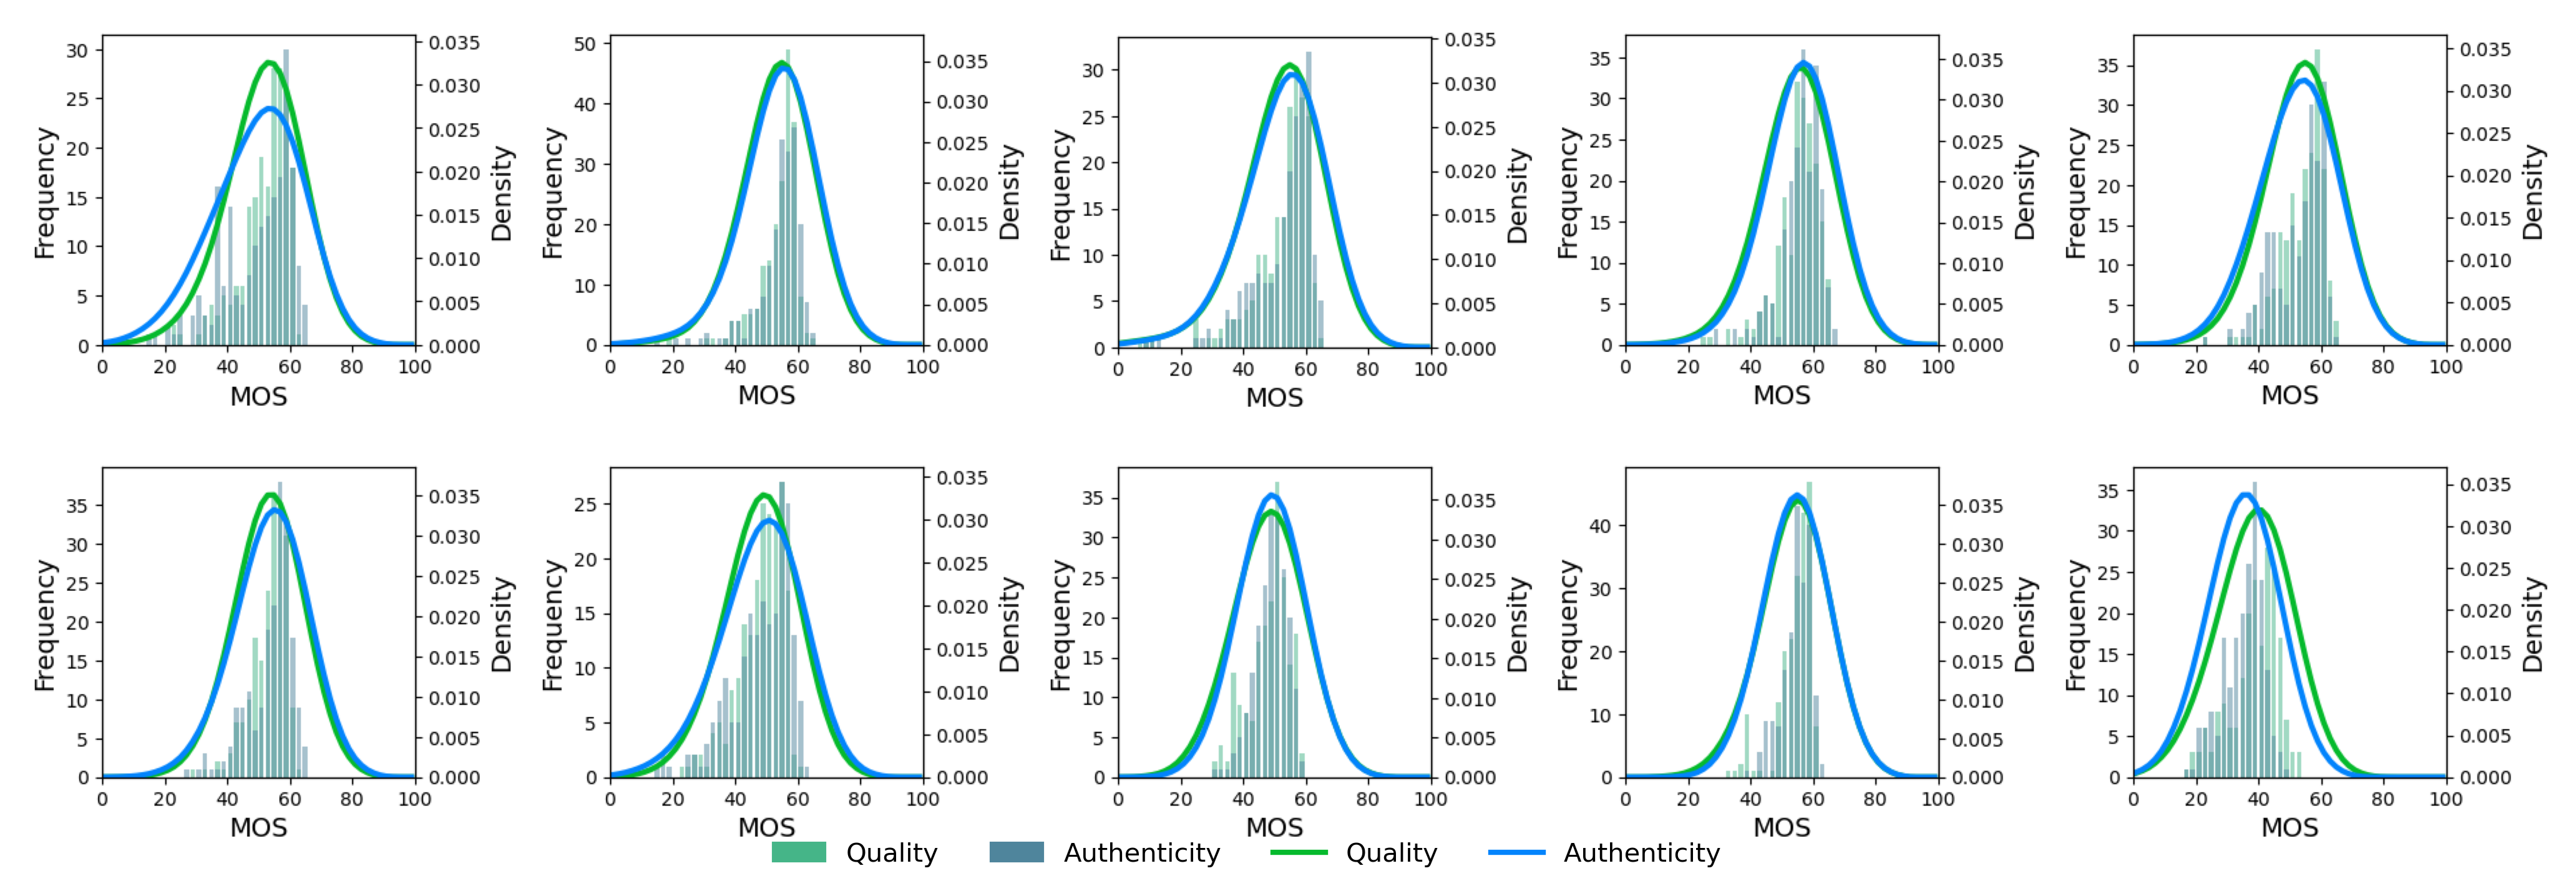}
    \vspace{-6mm}
    \caption{Mean Opinion Score (MOS) distribution histograms and kernel density curves of Gen3DHF dataset. It includes two dimensions: Quality MOS and Authenticity MOS. Each dimension contains a total of 2,000 MOS values.} 
     \vspace{-1mm}
    \label{appendix_mos}
\end{figure*}
