# Supplementary material for: LMME3DHF: Benchmarking and Evaluating Multimodal 3D Human Face Generation with LMMs
Source: arXiv:2504.20466 source file (2025-08-05)
Supplement: Supplementary file 9 [file model_url.tex]

\begin{table*}[t]
\centering
  \caption{An overview and URLs of the 3D human faces generation models.}
  \label{model_url}
  % \vspace{-2mm}
    
  \resizebox{0.9\textwidth}{!}{
    \begin{tabular}{l|c|c|c}
    \toprule
     Models & Year & Resolution & URL
     \\
    \midrule 
    EG3D~\cite{chan2022efficient} & 2022 & 512$\times$512 & \url{https://github.com/NVlabs/eg3d}
    \\
    PanoHead~\cite{an2023panohead} & 2023 & 1024$\times$1024 & \url{https://github.com/SizheAn/PanoHead}
    \\
    Next3D~\cite{sun2023next3d} & 2023 & 1024$\times$1024 & \url{https://github.com/MrTornado24/Next3D}
    \\
    AniFaceGAN~\cite{wu2022anifacegan} & 2022 & 512$\times$512 & \url{https://github.com/YueWuHKUST/AniFaceGAN}
    \\
    AniPortraitGAN~\cite{wu2023aniportraitgan} & 2023 & 512$\times$512 & \url{https://github.com/YueWuHKUST/AniPortraitGAN}
    \\
    Portrait4D~\cite{deng2024portrait4d} & 2024 & 1024$\times$1024 & \url{https://github.com/YuDeng/Portrait-4D}
    \\
    Portrait4D-v2~\cite{deng2024portrait4dv2} & 2024 & 1024$\times$1024 & \url{https://github.com/YuDeng/Portrait-4D}
    \\
    StyleSDF~\cite{or2022stylesdf} & 2022 & 1024$\times$1024 & \url{https://github.com/royorel/StyleSDF}
    \\
    VoxGRAF~\cite{schwarz2022voxgraf} & 2022 & 512$\times$512 & \url{https://github.com/autonomousvision/voxgraf}
    \\
    MVCGAN~\cite{zhang2022multi} & 2022 & 1024$\times$1024 & \url{https://github.com/Xuanmeng-Zhang/MVCGAN}
    \\
    cGOF~\cite{sun2022controllable} & 2022 & 512$\times$512 & \url{https://github.com/keqiangsun/cGOF}
    \\
    \bottomrule
  \end{tabular}}
    % \vspace{-3mm}
\end{table*}
