# Supplementary material for: LMME3DHF: Benchmarking and Evaluating Multimodal 3D Human Face Generation with LMMs
Source: arXiv:2504.20466 source file (2025-08-05)
Supplement: Supplementary file 11 [file saliency_predict_example.tex]

\begin{figure*}[!h]
    \centering
    \includegraphics[width=0.9\textwidth]{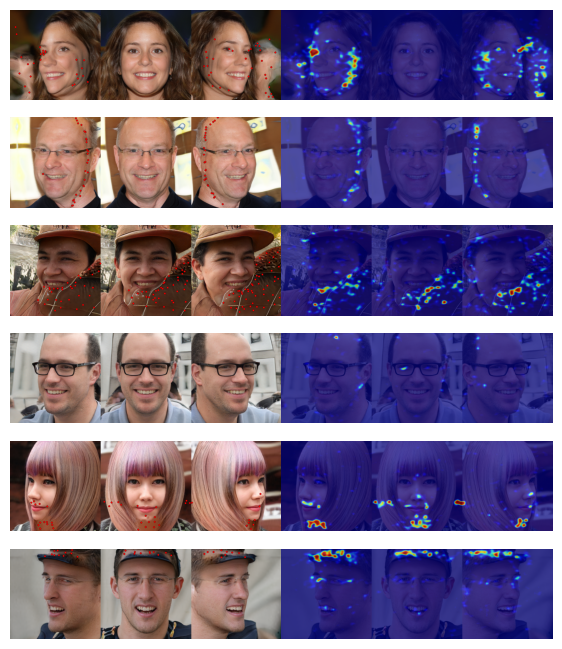}
    \caption{Examples of predicted saliency maps generated by our saliency decoder.} 
     \vspace{-1mm}
    \label{saliency_predict_example}
\end{figure*}
