# Supplementary material for: LMME3DHF: Benchmarking and Evaluating Multimodal 3D Human Face Generation with LMMs
Source: arXiv:2504.20466 source file (2025-08-05)
Supplement: Supplementary file 13 [file ui2.tex]

\begin{figure*}[!h]
	\centering
	\includegraphics[width=0.9\linewidth]{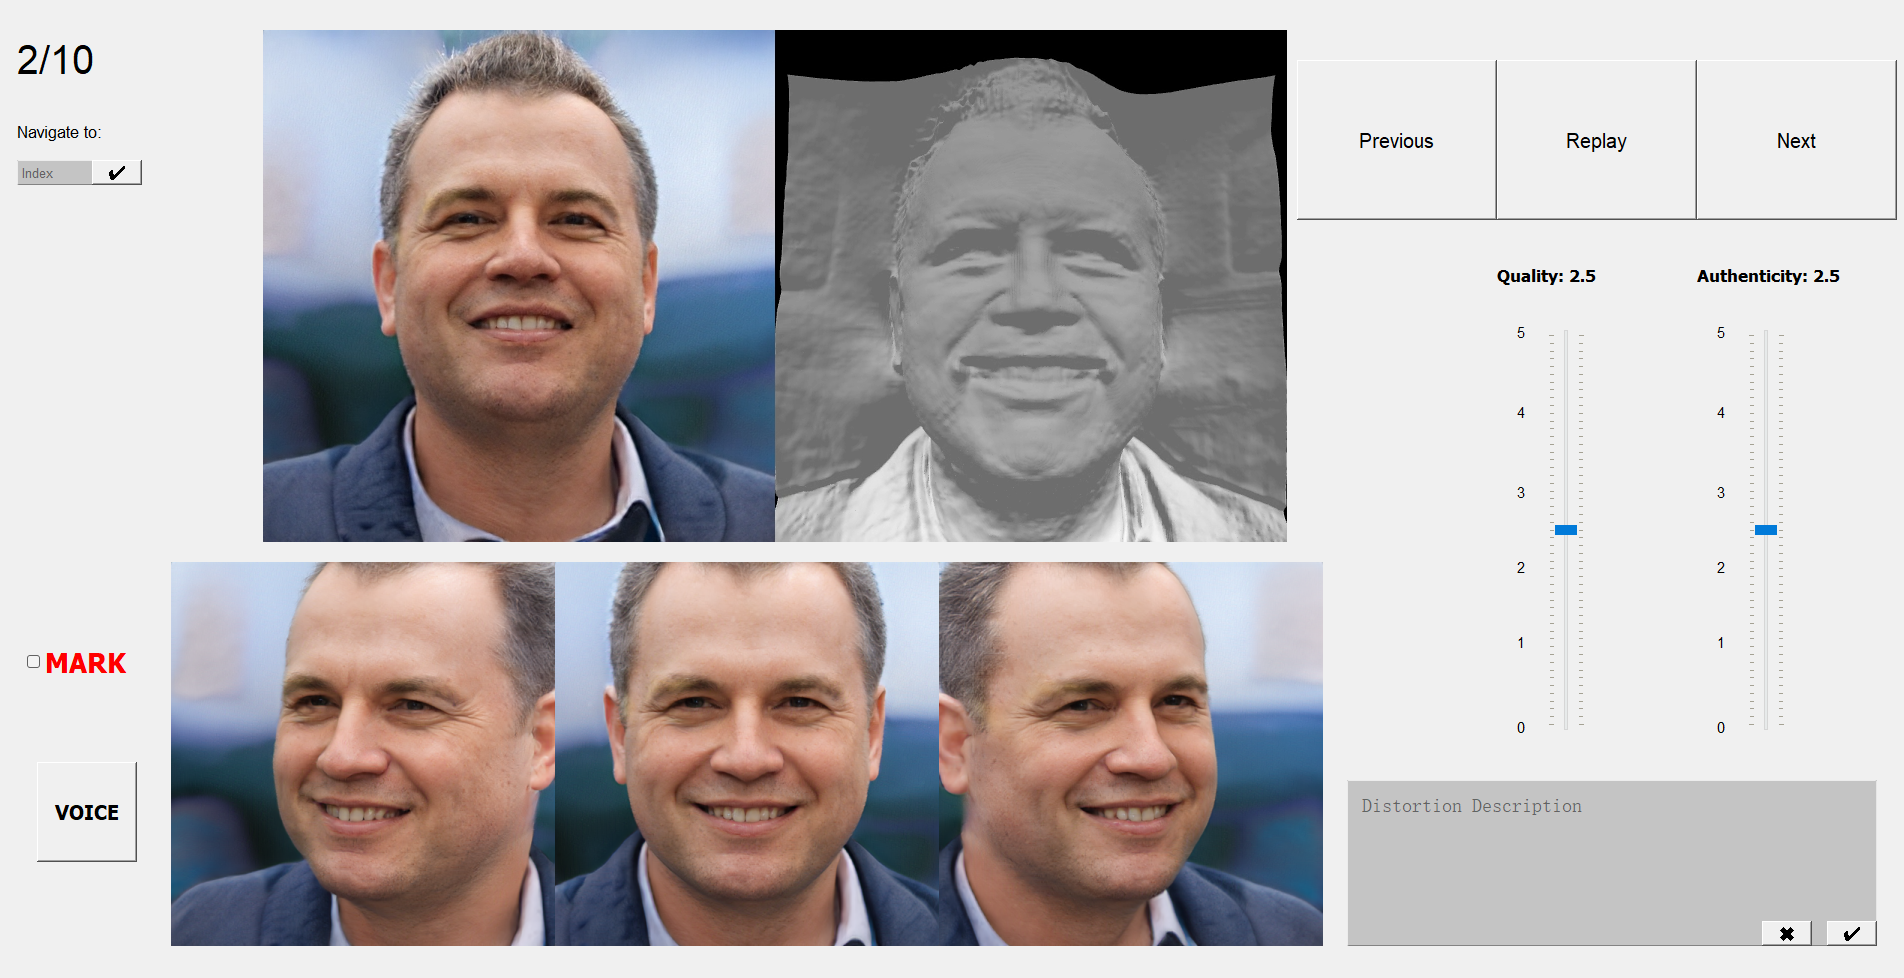}
	\caption{An example of the complex task annotation interface for human evaluation.}
	\label{ui2}
\end{figure*}
