# Supplementary material for: LMME3DHF: Benchmarking and Evaluating Multimodal 3D Human Face Generation with LMMs
Source: arXiv:2504.20466 source file (2025-08-05)
Supplement: Supplementary file 14 [file distortion_sample.tex]

\begin{figure}[!h]
    \centering
    \includegraphics[width=\linewidth]{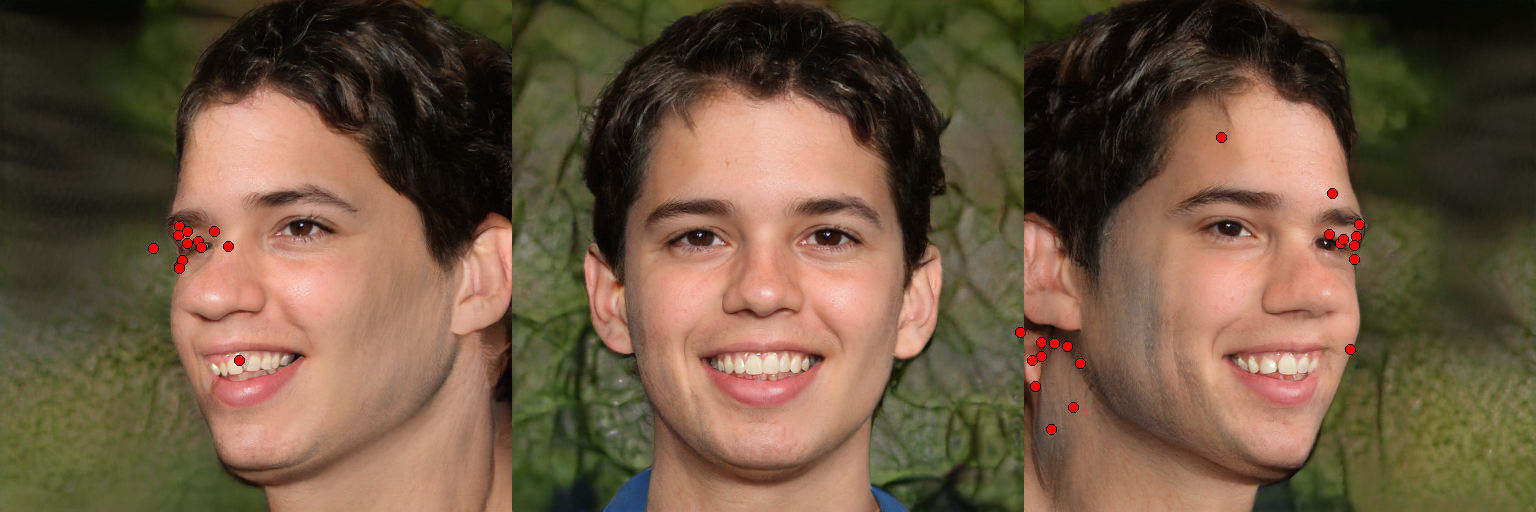}
    \caption{An example of distortion marks.} 
    \vspace{-3mm}
    \label{distortion_sample}
\end{figure}
